# Supplementary material for: Charge transfer of polyatomic molecules in ion-atom hybrid traps: Stereodynamics in the millikelvin regime
Source: arXiv:2303.15327 ancillary file (2023-07-11)
Supplement: Supplementary file 1 [file sm.pdf]

# Charge transfer of polyatomic molecules in ion-atom hybrid traps: Stereodynamics in the millikelvin regime

## Supplemental material

Alexandre Voute,[1,2,*] Alexander Dörfler,[3] Laurent Wiesenfeld,[2]
Olivier Dulieu,[2] Fabien Gatti,[1] Daniel Peláez,[1] and Stefan Willitsch[3,†]

[1] *Université Paris-Saclay, CNRS, Institut des Sciences Moléculaires d'Orsay, 91405, Orsay, France.*
[2] *Université Paris-Saclay, CNRS, Laboratoire Aimé-Cotton, 91405, Orsay, France.*
[3] *Department of Chemistry, University of Basel, Klingelbergstrasse 80, 4056 Basel, Switzerland*

(Dated: June 30, 2023)

## I. COMPUTATIONAL DETAILS

All the computations in this work were carried out with the Molpro quantum chemistry package [1–3].

*a. Asymptotic energies* Fig. S-1 gives an overview of all the asymptotic channels, in their ground and excited states. Ground-state energies were evaluated by computing energies of the fragments with the CCSD(T) method [4, 5], using the aug-cc-pVTZ basis set [6, 7] of the elements N and H and the aug-cc-pwCVTZ-PP basis set [8] for Rb. Energies of the asymptotic channels in other excited states are obtained by adding available experimental or theoretical values from the literature, listed in Table S-I, to the ground state energies computed in this work. As mentioned in the main text, the Fig. S-1 shows that the only thermodynamically accessible channels are $N_2 + H + Rb^+$, $N_2Rb^+ + H$ and $HRb^+ + N_2$ in the ground state.

*b. Potential curves of isolated $N_2H$ and $N_2H^+$* The PECs shown in Fig. 2 in the main text are obtained by computing the potentials of isolated $N_2H$ and $N_2H^+$ using the multi-reference configuration interaction (MRCI) method [15–17] with single and double excitations and the aug-cc-pVTZ basis set, using a reference wavefunction constructed with the dynamically-weighted state-averaged complete-active-space self-consistent-field (SW-SA-CASSCF) method

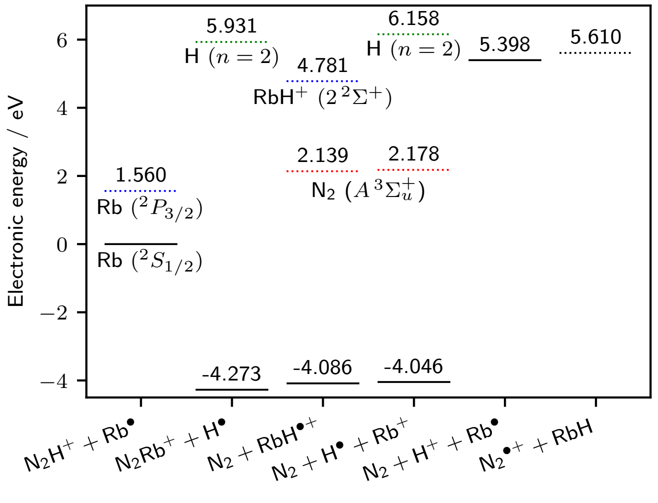


FIG. S-1. Asymptotic electronic energies of the $[N_2H{-}Rb]^+$ system. Solid lines : Computed *ab initio* CCSD(T) ground state energies. Dashed lines : Energies estimated from CCSD(T) ground state values from this work and other excitation or ionization energies from the literature of the indicated fragment, see Table S-I. In particular $E({N_2}^+ + RbH) = E(N_2 + H + Rb^+) - E_i(Rb) + E_i(N_2) - D_e(RbH)$.

* Corresponding author: alexandre.voute@universite-paris-saclay.fr
† Corresponding author: stefan.willitsch@unibas.ch

| Quantity | Name | Value / eV | Ref. | |
|---|---|---|---|---|
| Rb $(5p)\,^2P_{3/2}$ excited state energy | $E_e$(Rb) | 1.589 049 8 | [9, 10] | Exp. |
| Rb ionization energy | $E_i$(Rb) | 4.177 128 | [9, 10] | Exp. |
| $N_2$ $A\,^3\Sigma_u^+$ excited state energy | $E_e(N_2)$ | 6.224 460 | [11] | Exp. |
| $N_2$ ionization energy | $E_i(N_2)$ | 15.581 | [12] | Exp. |
| $RbH^+$ $2\,^2\Sigma^+$ excited state energy | $E_e(RbH^+)$ | 8.867 | [13] | Theory |
| RbH $X\,^1\Sigma^+$ ground state well depth | $D_e$(RbH) | 1.748 03 | [14] | Theory |

TABLE S-I. Values from the literature of energies used for the estimates shown in Fig. S-1. All values are given with respect to the ground state energy of the concerned atom or molecule. For molecules, they refer to the equilibrium geometry in the specified state.

[18–21]. For the neutral $N_2H$, a full-valence CAS of 11 electrons distributed over 9 active molecular orbitals (MOs) was used to compute two states of symmetry $A'$ and one of symmetry $A''$ within the $C_s$ point group. The the kink in the curve of state $2A'$ at $r = 2.6$ Å, as can be seen in Fig. 2 of the main text, is caused by the presence of another high-energy eigenstate of $N_2H$ of different character which is computed for $r > 2.6$ Å. It can be overlooked since, for large $r$, the excited states are well above the threshold and their energy is not required to be known with accuracy. Dynamical weighting prevents the kink to appear also in the ground state curve. For the cation, only the ground state was computed with standard CASSCF with only 10 active electrons. The PECs of $N_2H + Rb^+$ and $N_2H^+ + Rb$ at infinite ion-atom separation, shown in Fig. 2 in the main text, are obtained by lowering the PEC of $N_2H^+$ by the ionization energy of Rb, with respect to that of $N_2H$.

*c. Full [$N_2HRb$]$^+$ PESs and MEDPs* The three-dimensional PESs of $[N_2H{-}Rb]^+$ is computed at with the DW-SA-CASSCF method, using the aug-cc-PVTZ basis set for $N_2H$ and the ECP36SDF effective core potential [22, 23] with (4s4p)/[2s2p] basis set and a suitable core-polarized potential for the Rb atom. The CAS in these calculations includes all valence MOs of $N_2H/N_2H^+$ as above, augmented by four Rydberg orbitals, and the $5s$ orbital of Rb. In total, 11 electrons are distributed over 14 active orbitals. The choice of the extremal angles $\theta = 0.01°$ and $\theta = 179.99°$ instead of their rounded values comes from the unfortunate fact that, for a strictly linear geometry of the tetra-atomic, the CASSCF optimization procedure does not find the dissociative state among the eigenstates of the electronic Hamiltonian, probably because of symmetry considerations. The MEDPs were obtained by numerical minimization of the square of the energy difference between states $2A'$ and $3A'$ against $r$ for a given choice of $R$ and $\theta$.

## II. ESTIMATES OF TRANSITION PROBABILITIES

Given an avoided crossing between two adiabatic potential energy curves $V_1$ and $V_2$, and their diabatic counterparts $W_{11}$ and $W_{22}$ crossing at $x^*$, the Landau-Zener transition probability from one adiabatic state to the other is given by:

$$P_{\mathrm{LZ}} = \exp\left(-\frac{2\pi}{\hbar}\frac{W_{12}^2}{v\Delta G}\right) \tag{1}$$

In Eq. (1), $W_{12} = (V_2(x^*) - V_1(x^*))/2$, the quantity $v$ is the local velocity of the system at the crossing and $\Delta G = |G_1(x^*) - G_2(x^*)|$, where $G_1$ and $G_2$ are the spatial derivatives of $W_{11}$ and $W_{22}$, respectively. The local velocity can be estimated with:

$$v = \sqrt{2E_{\mathrm{loc}}/\mu} \tag{2}$$

The value of $E_{\mathrm{loc}}$ used for the estimates depends on the considered motion coordinate.

The diabatic transition depicted in Fig. 4 (a) in the main text involves essentially the collision coordinate $R$, so the local velocity can be retrieved from the kinetic energy at the avoided crossing position gained along the attractive potential from infinite separation, i.e.:

$$E_{\mathrm{loc}} = -V_{3A'}(x^*) \tag{3}$$

where $\mu$ is the reduced mass the $N_2H^+ + Rb$ system.

Next, the process of staying adiabatically in state $2A'$ addressed in Fig. 4 (b), i.e. where the charge transfer occurs, is mainly driven by the dissociation coordinate $r$. This adiabatic passage is favored by the increasing energy gap at the avoided crossing between adiabatic states $2A'$ and $3A'$. Along this coordinate, it is the vibrational zero-point energy contribution of the $N_2{-}H^+$ stretching motion ($\tilde{\nu} = 2257.867$ cm$^{-1}$ [24]) which is mainly involved in the dynamics across the avoided crossing, i.e.:

$$E_{\mathrm{loc}} = hc\tilde{\nu}/2 \tag{4}$$

where this time $\mu$ in Eq. (2) is the reduced mass of $N_2 + H$.

A summary of the diabatic transition probabilities computed as described above, in particular for $\theta = 120°$, is given in Table S-II. In both estimates, the $W_{12}$ term is evaluated from the MEDP and the gradients are computed from 1D cuts along the considered propagation coordinate.

| Propagation coord. | MEDP Position | | | | | | | |
|---|---|---|---|---|---|---|---|---|
| | $r$/Å | $R$/Å | $\theta$/° | $\Delta G$ / a.u. | $W_{12}$ / a.u. | $E_{\mathrm{loc}}$ / a.u. | $v$ / a.u. | $P_{\mathrm{LJ}}$ |
| $R$ | 1.5826 | 15.0 | 180 | $1.070 \times 10^{-4}$ | $9.7728 \times 10^{-7}$ | $1.5523 \times 10^{-4}$ | $8.8745 \times 10^{-5}$ | **1.000** |
| | 1.6076 | 8.5 | 180 | $1.120 \times 10^{-3}$ | $4.7206 \times 10^{-4}$ | $1.3561 \times 10^{-3}$ | $2.6231 \times 10^{-4}$ | 0.304 |
| | 1.6296 | 6.5 | 180 | $2.107 \times 10^{-3}$ | $2.6735 \times 10^{-3}$ | $2.4485 \times 10^{-3}$ | $3.5246 \times 10^{-4}$ | $2.710 \times 10^{-7}$ |
| | 1.5815 | 13.0 | 120 | $2.723 \times 10^{-4}$ | $5.2324 \times 10^{-5}$ | $3.9363 \times 10^{-4}$ | $1.4132 \times 10^{-4}$ | **0.894** |
| | 1.6075 | 8.0 | 120 | $1.600 \times 10^{-3}$ | $1.8432 \times 10^{-3}$ | $2.0057 \times 10^{-3}$ | $3.1900 \times 10^{-4}$ | $2.879 \times 10^{-5}$ |
| | 1.6299 | 6.5 | 120 | $2.528 \times 10^{-3}$ | $3.2654 \times 10^{-3}$ | $4.0105 \times 10^{-3}$ | $4.5108 \times 10^{-4}$ | $4.179 \times 10^{-7}$ |
| | 1.5806 | 10.0 | 90 | $9.490 \times 10^{-4}$ | $1.5758 \times 10^{-3}$ | $8.0078 \times 10^{-4}$ | $2.0156 \times 10^{-4}$ | $1.391 \times 10^{-9}$ |
| | 1.6072 | 7.5 | 90 | $2.716 \times 10^{-3}$ | $7.3834 \times 10^{-3}$ | $1.8101 \times 10^{-3}$ | $3.0305 \times 10^{-4}$ | $6.564 \times 10^{-46}$ |
| | 1.6294 | 6.5 | 90 | $3.879 \times 10^{-3}$ | $1.0933 \times 10^{-2}$ | $3.0809 \times 10^{-3}$ | $3.9536 \times 10^{-4}$ | $6.660 \times 10^{-54}$ |
| $r$ | 1.5826 | 15.0 | 180 | 0.1112 | $9.7728 \times 10^{-7}$ | 0.139 96 | $2.4086 \times 10^{-3}$ | 1.000 |
| | 1.6076 | 8.5 | 180 | 0.1345 | $4.7206 \times 10^{-4}$ | ” | ” | *0.999* |
| | 1.6296 | 6.5 | 180 | 0.1761 | $2.6735 \times 10^{-3}$ | ” | ” | *0.974* |
| | 1.5815 | 13.0 | 120 | 0.1092 | $5.2324 \times 10^{-5}$ | ” | ” | 1.000 |
| | 1.6075 | 8.0 | 120 | 0.1334 | $1.8432 \times 10^{-3}$ | ” | ” | *0.984* |
| | 1.6299 | 6.5 | 120 | 0.1641 | $3.2654 \times 10^{-3}$ | ” | ” | *0.959* |
| | 1.5806 | 10.0 | 90 | 0.1089 | $1.5758 \times 10^{-3}$ | ” | ” | 0.985 |
| | 1.6072 | 7.5 | 90 | 0.1462 | $7.3834 \times 10^{-3}$ | ” | ” | 0.784 |
| | 1.6294 | 6.5 | 90 | 0.1820 | $1.0933 \times 10^{-2}$ | ” | ” | 0.652 |

TABLE S-II. Landau-Zener diabatic transition probabilities estimated with Eq. (1). Half-energy gaps $W_{12}$ are computed at the specified positions on the MEDP. The local kinetic energy $E_{\mathrm{loc}}$ is and collision energies (for propagation along $R$). Gradient differences are estimated from the 1D cuts along the specified motion coordinate which are the closest to the point on the MEDP. Values in **boldface** are those related to the first diabatic transition indicated in Fig. 4 (a) in the main text. Values in *italic* refer to the adiabatic transition indicated in Fig. 4 (b) in the main text.

## III. TIMESCALES ESTIMATES

### A. Approaching time vs. rotational period of $N_2H^+$

We estimate and compare here the timescales of rotation of $N_2H^+$ against that of the approach of Rb for which the PES is considered as being no longer invariant with respect to the angle of attack $\theta$. The anisotropy of the PES of state $3A'$ can be appreciated for $R < 25$ Å. The typical approaching time from the most unfavorable angle of attack $\theta = 0°$, where the well depth of the PEC of state $3A'$ is 0.034 eV, can thus be given by estimating how long it takes to the system to evolve from $R_+ = 25$ Å to the turning point at $R_- = 10$ Å. The average speed in this range is calculated as:

$$\left\langle \dot{R} \right\rangle = \frac{1}{\Delta R} \int_{R_-}^{R_+} \sqrt{\frac{2E(R)}{\mu}}\, \mathrm{d}R \tag{5}$$

where $\Delta R = R_+ - R_-$, $\mu$ is the reduced mass of the $N_2H^+ + Rb$ system and $E(R) = -V_{3A'}(r = r_{\rm eq}, R, \theta = 0°)$. The typical approaching time $\tau_a$ can be estimated with:

$$\tau_a = \frac{\Delta R}{\left\langle \dot{R} \right\rangle} \tag{6}$$

The obtained numerical value is $\tau_a \approx 5$ ps.

The rotational constant of $N_2H^+$ is $\tilde{B} = 1.5539$ cm$^{-1}$ (from Ref. [25]). In a Boltzmann distribution for this cation at room temperature, the most populated rotational state is $J = 10$. From the classical and quantum rotational energy of a rigid rotor, we have:

$$E_{\rm rot} = hc\tilde{B}J(J+1) = \frac{1}{2}I\omega^2 \tag{7}$$

with $\tilde{B} = \hbar/(4\pi cI)$ and $\omega = 2\pi/T_{\rm rot}$. The rotational period $T_{\rm rot}$ is thus given by:

$$T_{\rm rot} = \frac{1}{2c\tilde{B}\sqrt{J(J+1)}} \tag{8}$$

For $J = 10$, the rotational period of $N_2H^+$ is $T_{\rm rot} \approx 1$ ps.

### B. Collision vs. $N_2{-}H^+$ stretching period

We estimate and compare the timescales of vibration of $N_2{-}H^+$ against that of the collision with Rb at $\theta = 120°$ after the diabatic transition occurring around $R = 13.5$ Å. This indicates "how frequently" the system can adiabatically leak through the avoided crossing along the $r$ coordinate in the region of short $R$ where the energy gap at the crossing widens.

The typical collision time $\tau_c$ can be calculated using Eq. (5) by setting $E(R) = -V_{2A'}(r = r_{\rm eq}, R, \theta = 120°)$, the upper bound $R_+ = 13.5$ Å and the the turning point $R_- = 3.75$ Å. An oscillation in this region is thus given by twice the time given in Eq. (6) that is $\tau_c = 2.26$ ps.

The experimental vibrational frequency of the $N_2{-}H^+$ stretching vibration is $\tilde{\nu} = 2257.867$ cm$^{-1}$ (from Ref. [24]). In the harmonic oscillator approximation, the vibrational period is given by:

$$T_{\rm vib} = 1/c\tilde{\nu} \tag{9}$$

which yields $T_{\rm vib} \approx 15$ fs.

## IV. POTENTIAL ENERGY SURFACES CONTOUR PLOTS AND MINIMUM ENERGY DIFFERENCE PATHS BETWEEN STATES INVOLVED IN CHARGE TRANSFER AT VARIOUS COLLISION ANGLES

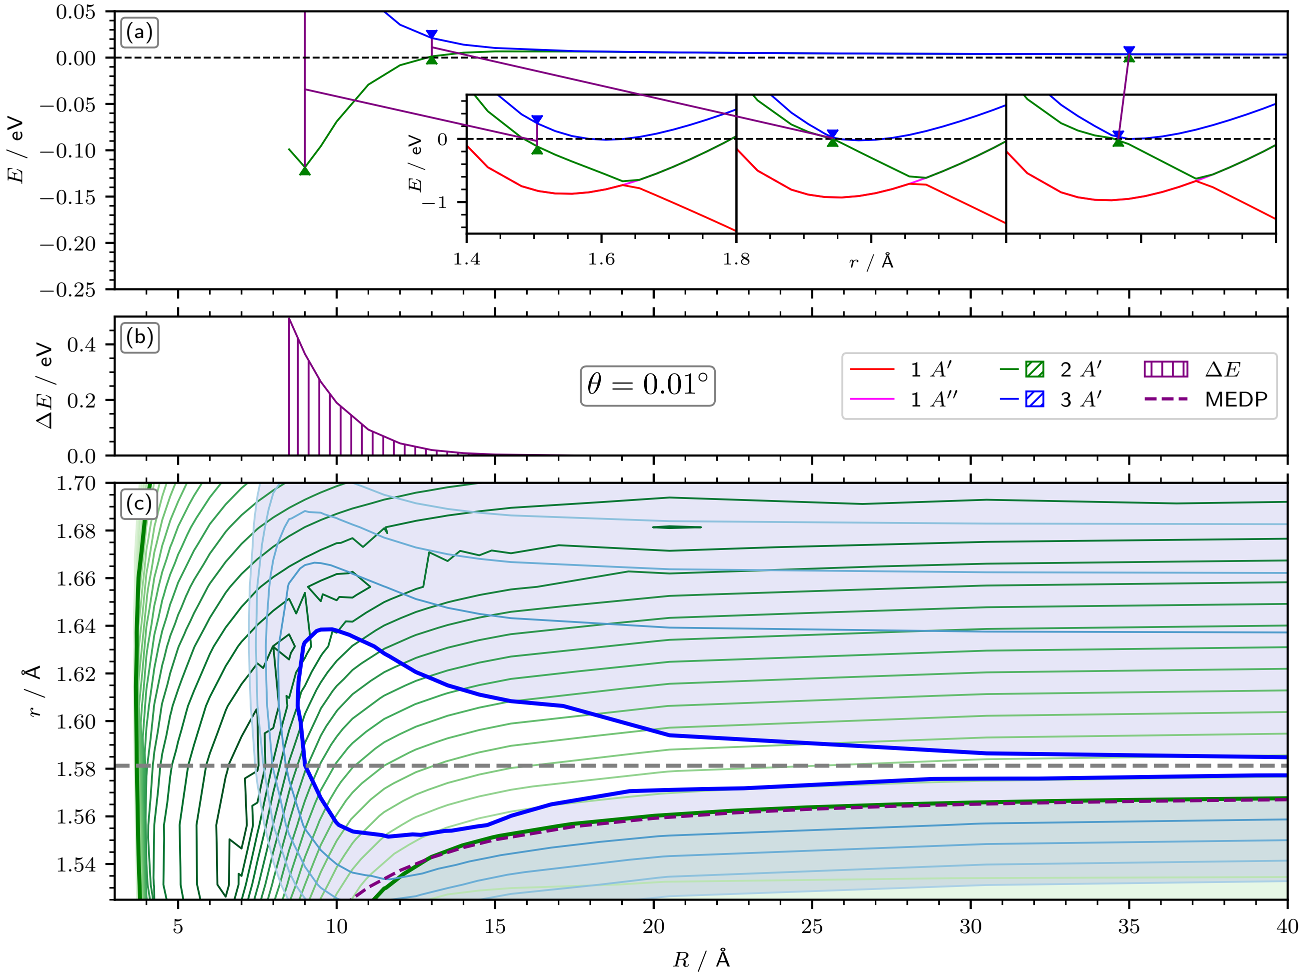


FIG. S-2. Potential energy landscape of the $N_2H^+ + Rb$ collisional system for $\theta = 0.01^\circ \approx 0^\circ$. (a) Energies of the states $2A'$ and $3A'$ along the minimum energy difference path (MEDP) projected along the $R$-axis. The insets display cuts of the PESs along the $r$ coordinate at selected values of $R$ corresponding to the abscissa of the triangular cursors in the main panel. The pairs of cursors in the panel and in each of the insets which are joined by a line correspond to the same points in energy and configuration space. (b) Energy difference between states $2A'$ and $3A'$ along the MEDP. (c) Contour plots of the PESs of states $2A'$ and $3A'$ as functions of $r$ and $R$. The thick green and blue contour lines correspond to the threshold energy $E = 0$ in those states, respectively. Other isoenergetic contours are traced every 0.05 eV. Shaded areas correspond to energy-forbidden regions of configuration space. The thick dashed grey line indicates the entrance asymptotic channel ($r = r_e, R \to \infty$). The dashed purple line is the MEDP for the given $\theta$ whose energies in the two states are given in panel (a). For simplicity, the PES of state $1A'$ is not shown in panel (c) but the seam of intersections between states $1A'$ and $2A'$ can be guessed from the irregularities in the green contours with the guidance of the insets in panel (a) and Fig. 4. Note that, for this collinear arrangement (Rb attacking on the H-side of $N_2H^+$), the MEDP remains in the energy-forbidden region and that the energy-allowed region in state $3A'$ is bounded at $R > 9$ Å.

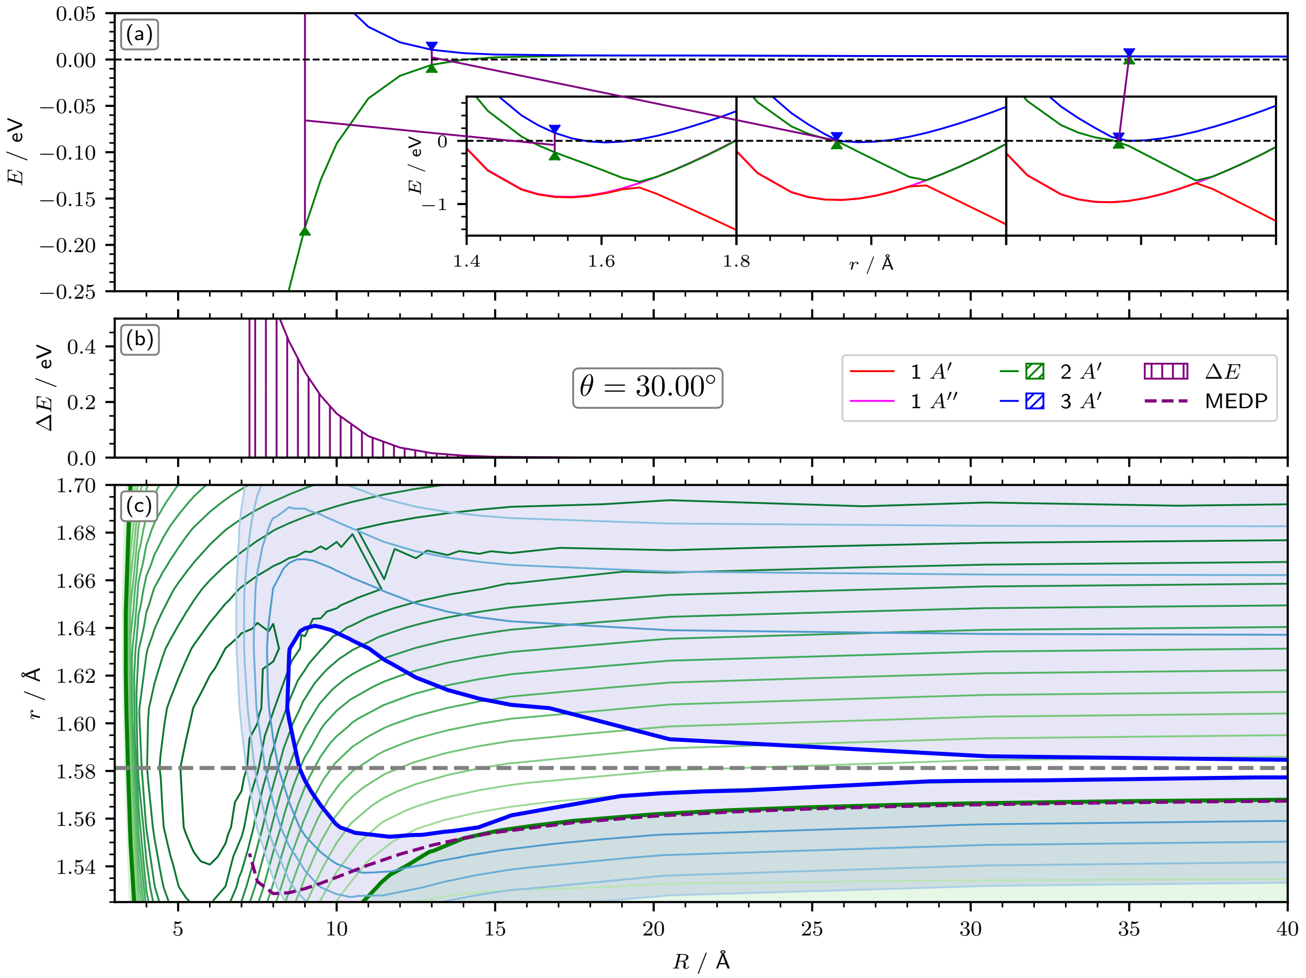


FIG. S-3. Same as Fig. S-2, for $\theta = 30^{\circ}$.

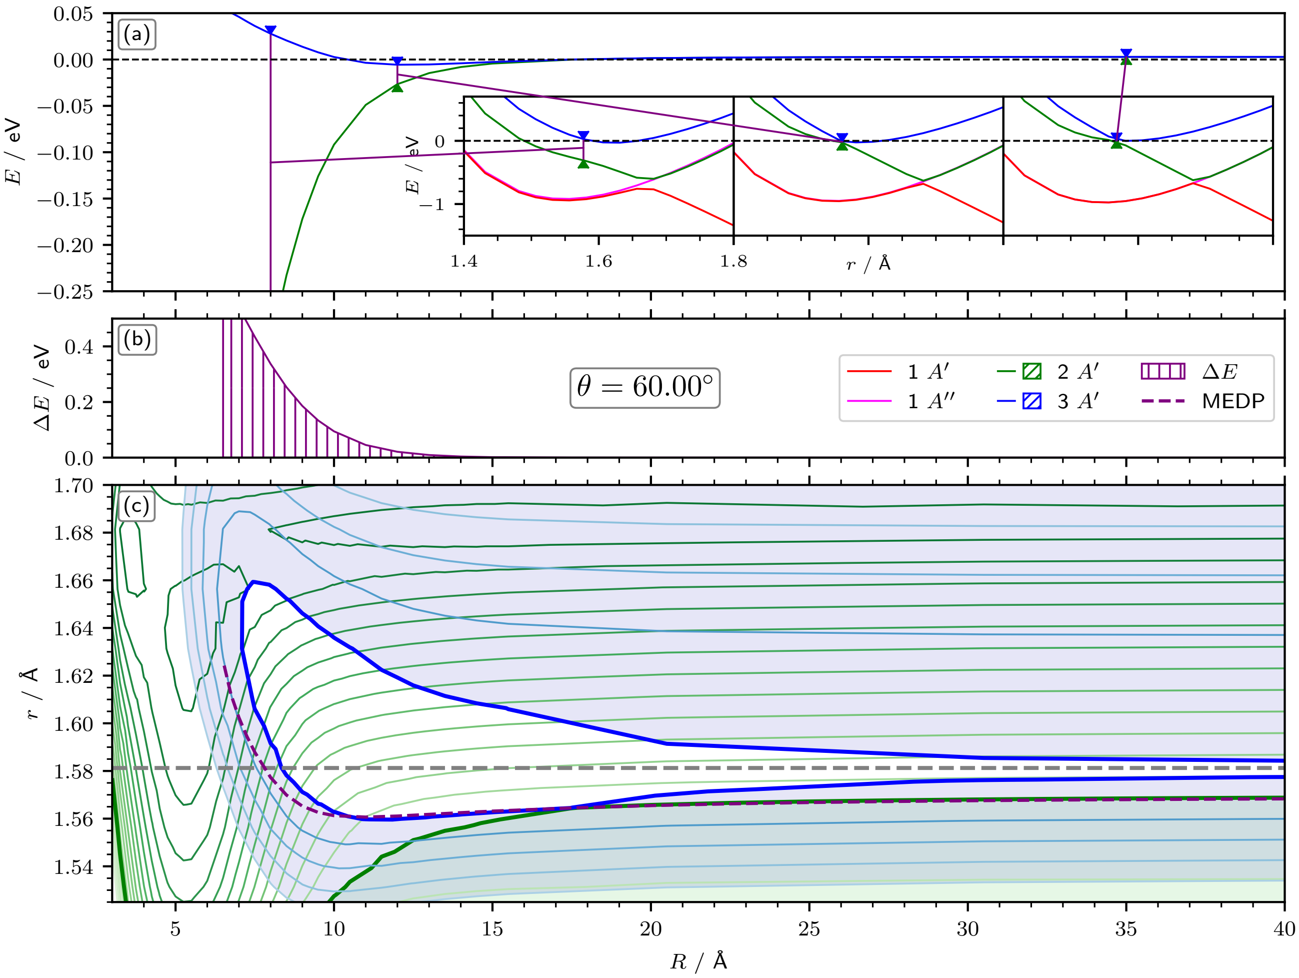


FIG. S-4. Same as Fig. S-2, for $\theta = 60^\circ$. Note in panel (c) that the MEDP is almost tangent to the $E = 0$ contour line and barely enters in the energy-allowed region in state $3A'$, as can be seen in panel (a).

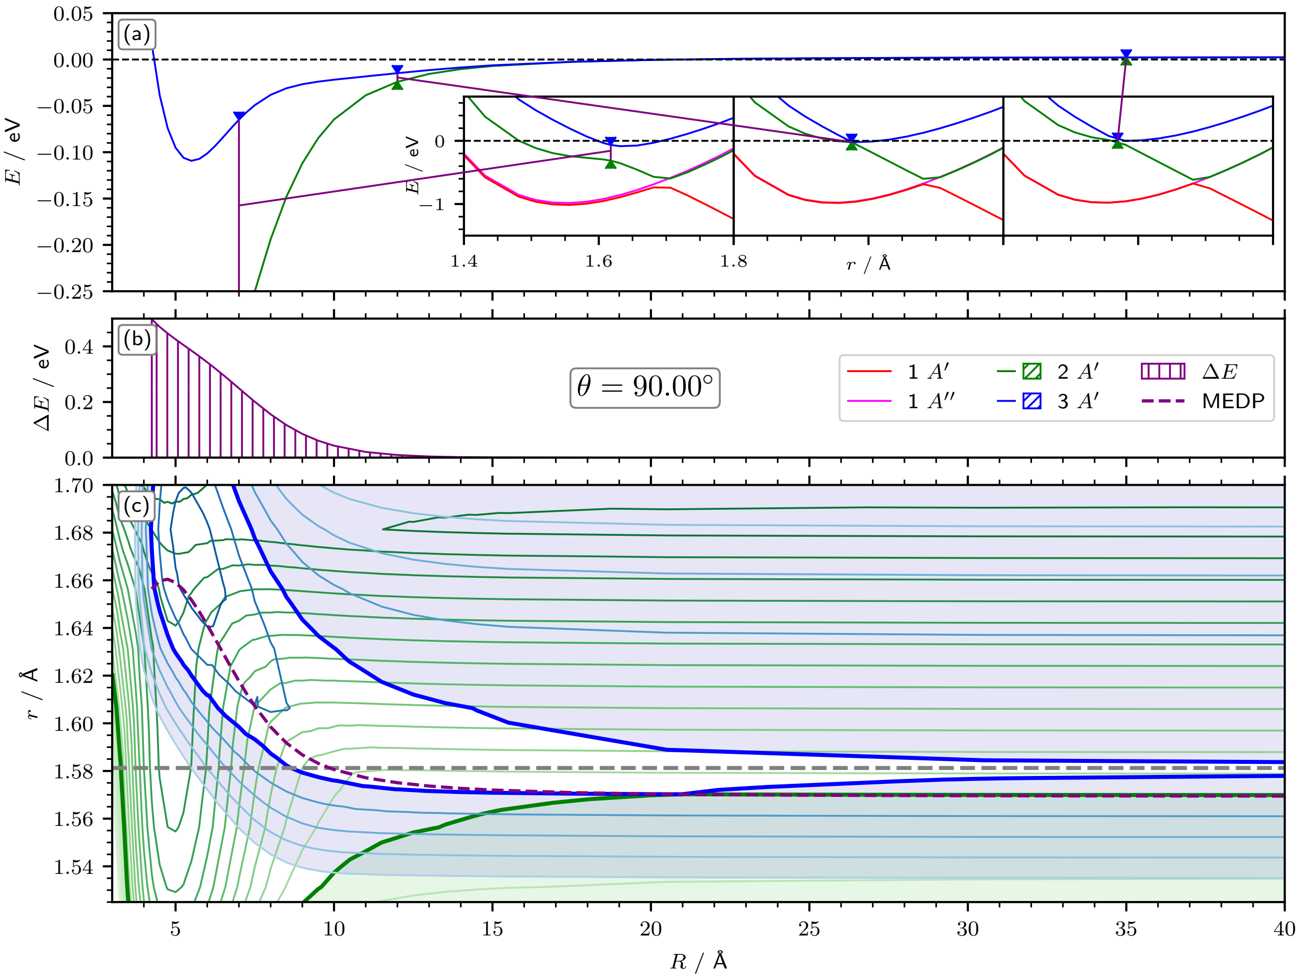


FIG. S-5. Same as Fig. S-2, for $\theta = 90°$.

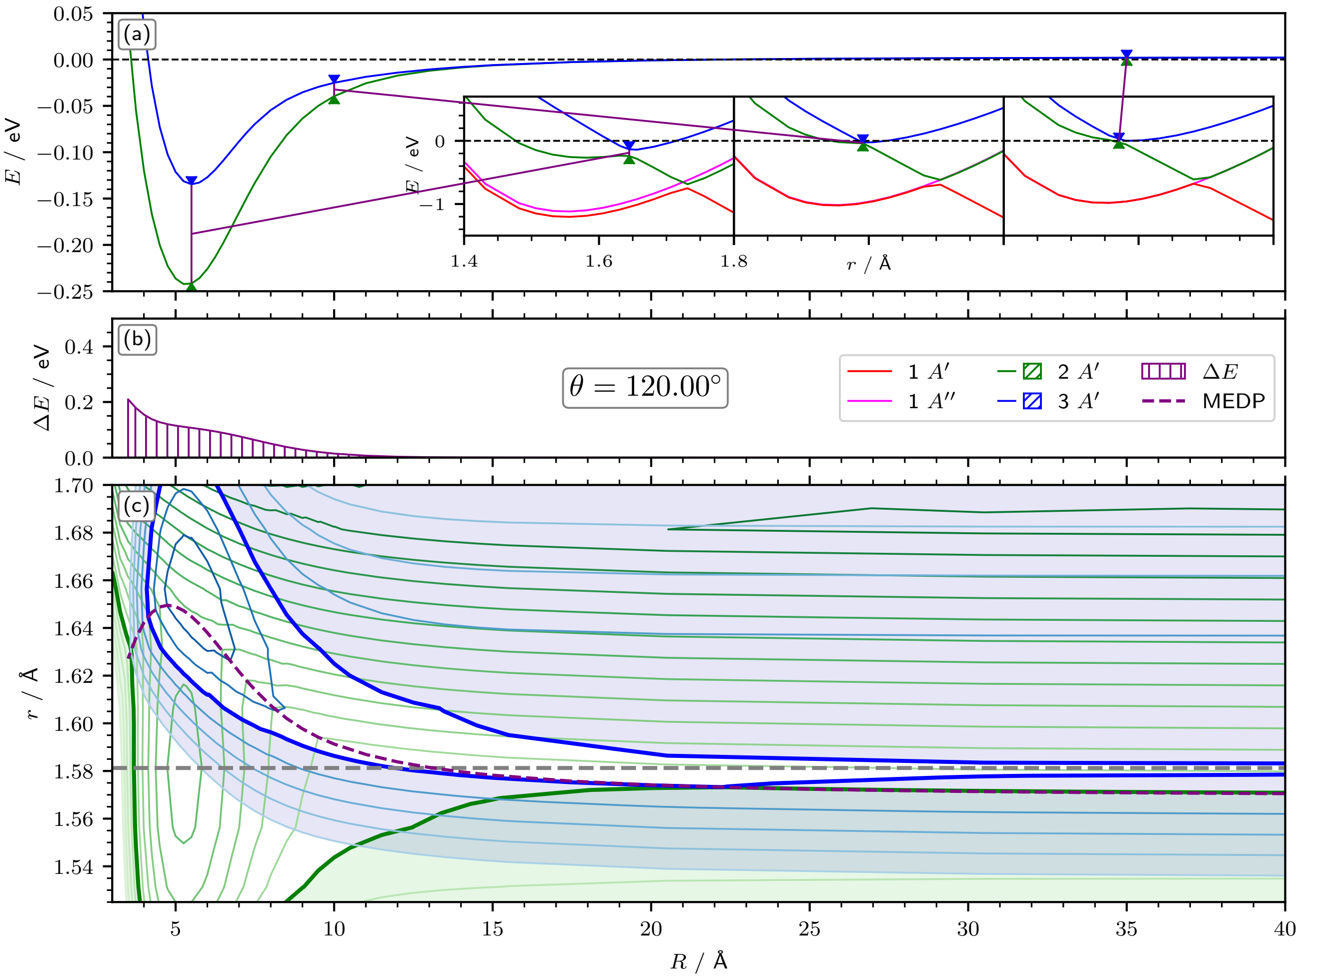


FIG. S-6. Same as Fig. S-2, for $\theta = 120°$. Note how, in contrast with Fig. S-2, the MEDP enters in the energy-allowed region of state $3A'$ (panel (c) ), significantly below the threshold energy (panel (a) ) and with a smaller energy gap between the two states (panel (b) ).

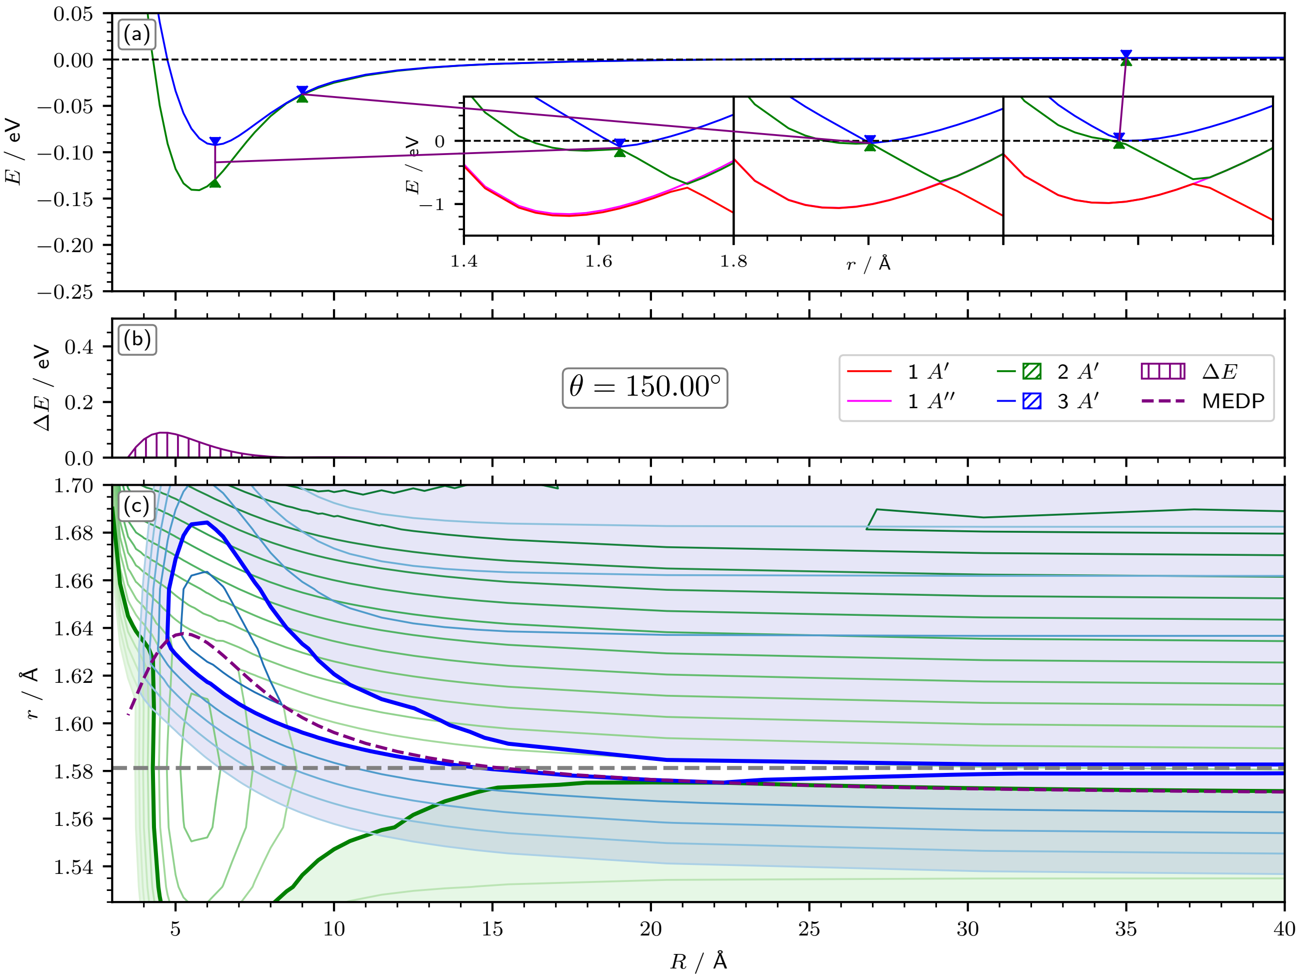


FIG. S-7. Same as Fig. S-2, for $\theta = 150°$.

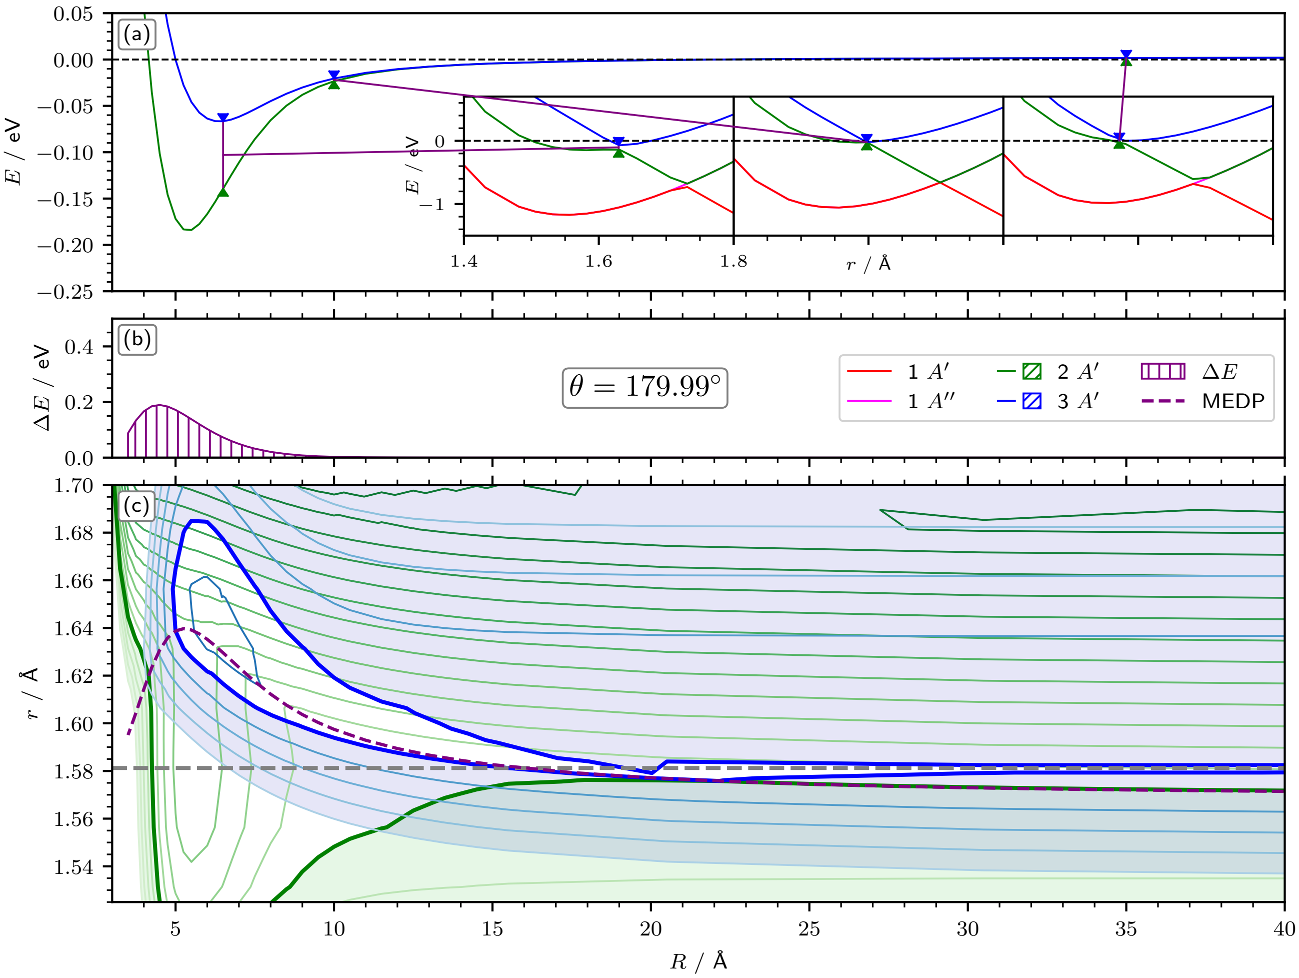


FIG. S-8. Same as Fig. S-2, for $\theta = 179.99^\circ$.

[1] H.-J. Werner, P. J. Knowles, G. Knizia, F. R. Manby, M. Schütz, P. Celani, W. Györffy, D. Kats, T. Korona, R. Lindh, A. Mitrushenkov, G. Rauhut, K. R. Shamasundar, T. B. Adler, R. D. Amos, S. J. Bennie, A. Bernhardsson, A. Berning, D. L. Cooper, M. J. O. Deegan, A. J. Dobbyn, F. Eckert, E. Goll, C. Hampel, A. Hesselmann, G. Hetzer, T. Hrenar, G. Jansen, C. Köppl, S. J. R. Lee, Y. Liu, A. W. Lloyd, Q. Ma, R. A. Mata, A. J. May, S. J. McNicholas, W. Meyer, T. F. M. III, M. E. Mura, A. Nicklass, D. P. O'Neill, P. Palmieri, D. Peng, K. Pflüger, R. Pitzer, M. Reiher, T. Shiozaki, H. Stoll, A. J. Stone, R. Tarroni, T. Thorsteinsson, M. Wang, and M. Welborn, MOLPRO, version 2022.1, a package of ab initio programs.

[2] H.-J. Werner, P. J. Knowles, G. Knizia, F. R. Manby, and M. Schütz, Molpro: a general-purpose quantum chemistry program package, WIREs Comput. Mol. Sci. **2**, 242 (2012).

[3] H.-J. Werner, P. J. Knowles, F. R. Manby, J. A. Black, K. Doll, A. Heßelmann, D. Kats, A. Köhn, T. Korona, D. A. Kreplin, Q. Ma, T. F. Miller, A. Mitrushchenkov, K. A. Peterson, I. Polyak, G. Rauhut, and M. Sibaev, The Molpro quantum chemistry package, J. Chem. Phys. **152**, 144107 (2020).

[4] K. Raghavachari, G. W. Trucks, J. A. Pople, and M. Head-Gordon, A fifth-order perturbation comparison of electron correlation theories, Chem. Phys. Lett. **157**, 479 (1989).

[5] C. Hampel, K. A. Peterson, and H.-J. Werner, A comparison of the efficiency and accuracy of the quadratic configuration interaction (QCISD), coupled cluster (CCSD), and Brueckner coupled cluster (BCCD) methods, Chem. Phys. Lett. **190**, 1 (1992).

[6] T. H. Dunning, Gaussian basis sets for use in correlated molecular calculations. I. The atoms boron through neon and hydrogen, J. Chem. Phys. **90**, 1007 (1989).

[7] R. A. Kendall, T. H. Dunning, and R. J. Harrison, Electron affinities of the first-row atoms revisited. Systematic basis sets and wave functions, J. Chem. Phys. **96**, 6796 (1992).

[8] J. G. Hill and K. A. Peterson, Gaussian basis sets for use in correlated molecular calculations. XI. Pseudopotential-based and all-electron relativistic basis sets for alkali metal (K-Fr) and alkaline earth (Ca–Ra) elements, J. Chem. Phys. **147**, 244106 (2017).

[9] I. Johansson, Spectra of the alkali metals in the lead-sulphide region, Ark. Fys. **20**, 135 (1961).

[10] J. E. Sansonetti, Wavelengths, Transition Probabilities, and Energy Levels for the Spectra of Rubidium (Rb I through Rb XXXVII), J. Phys. Chem. Ref. Data **35**, 301 (2006).

[11] R. Miller, The absolute energy of the $A^3\Sigma_u^+$ state of nitrogen, J. Mol. Spec. **19**, 185 (1966).

[12] T. Trickl, E. F. Cromwell, Y. T. Lee, and A. H. Kung, State-selective ionization of nitrogen in the $X^2\Sigma_g^+$ $v_+ = 0$ and $v_+ = 1$ states by two-color $(1+1)$ photon excitation near threshold, J. Chem. Phys. **91**, 6006 (1989).

[13] L. Yan, Y. Qu, C. Liu, J. Wang, and R. J. Buenker, Ab initio many-electron study for the low-lying states of the alkali hydride cations in the adiabatic representation, J. Chem. Phys. **136**, 124304 (2012).

[14] M. Aymar, J. Deiglmayr, and O. Dulieu, Systematic trends in electronic properties of alkali hydrides, Can. J. Phys. **87**, 543 (2009).

[15] H.-J. Werner and P. J. Knowles, An Efficient Internally Contracted Multiconfiguration Reference CI Method, J. Chem. Phys. **89**, 5803 (1988).

[16] P. J. Knowles and H.-J. Werner, An Efficient Method for the Evaluation of Coupling Coefficients in Configuration Interaction Calculations, Chem. Phys. Lett. **145**, 514 (1988).

[17] P. J. Knowles and H.-J. Werner, Internally contracted multiconfiguration-reference configuration interaction calculations for excited states, Theor. Chem. Acc. **84**, 95 (1992).

[18] M. P. Deskevich, D. J. Nesbitt, and H.-J. Werner, Dynamically weighted multiconfiguration self-consistent field: Multistate calculations for $F + H_2O \longrightarrow HF + OH$ reaction paths, J. Chem. Phys. **120**, 7281 (2004).

[19] H. Werner and P. J. Knowles, A second order multiconfiguration SCF procedure with optimum convergence, J. Chem. Phys. **82**, 5053 (1985).

[20] P. J. Knowles and H.-J. Werner, An Efficient Second Order MCSCF Method for Long Configuration Expansions, Chem. Phys. Lett. **115**, 259 (1985).

[21] D. A. Kreplin, P. J. Knowles, and H.-J. Werner, Second-order MCSCF optimization revisited. I. Improved algorithms for fast and robust second-order CASSCF convergence, J. Chem. Phys. **150**, 194106 (2019).

[22] L. von Szentpály, P. Fuentealba, H. Preuss, and H. Stoll, Pseudopotential calculations on ${Rb_2}^+$, ${Cs_2}^+$, $RbH^+$, $CsH^+$ and the mixed alkali dimer ions, Chem. Phys. Lett. **93**, 555 (1982).

[23] P. Fuentealba, H. Stoll, L. von Szentpaly, P. Schwerdtfeger, and H. Preuss, On the reliability of semi-empirical pseudopotentials: simulation of Hartree-Fock and Dirac-Fock results, J. Phys. B **16**, L323 (1983).

[24] S. C. Foster and A. R. W. McKellar, The $\nu_3$ fundamental bands of ${HN_2}^+$ , ${DN_2}^+$ , and $DCO^+$, J. Chem. Phys. **81**, 3424 (1984).

[25] T. Amano, T. Hirao, and J. Takano, Submillimeter-wave spectroscopy of ${HN_2}^+$ and ${DN_2}^+$ in the excited vibrational states, J. Mol. Spec. **234**, 170 (2005).
